# Supplementary material for: Proof-of-Prestige: A Useful Work Reward System for Unverifiable Tasks
Source: arXiv:1905.03016 source file (2019-05-08)
Supplement: Supplementary file 1 [file appendix.tex]

\appendix

%Restart theorem counter
\counterwithin{theorem}{section}

\section{Proofs}\label{sec:proofs}

\begin{theorem}Each user has no prestige gain incentives to divide their coins into multiple identities.
\end{theorem}
\begin{proof}Let user $i$ divide her coins into $1,2,...,k$ identities according to $C_{i,1},C_{i,2},...,C_{i,k}$ respectively, such that $\sum\limits_{q=1}^kC_{i,q}=C_{i}$. Then the aggregated prestige of multiple identities upon time-slot $t$ is:
\begin{align*}
P_{i,1}^t+P_{i,2}^t+...+P_{i,k}^t&=\sum\limits_{q=1}^kC_{i,q}\sum\limits_{j=1}^{t}\sum\limits_{n=0}^{j-1}(-1 d)^n,\\
&=P_i^t.
\end{align*}That is, the total prestige generated by multiple identities equals the prestige that would have been normally achieved.
\end{proof}

\begin{theorem}There is no additional overall prestige gain incentives caused by prestige transfers between users.
\end{theorem}
\begin{proof}We denote by $P_i^t$, $P_j^t$ the prestige of contributor $i$ and beneficiary $j$ when there is no prestige transfer from $i$ to $j$ and by  $\bar{P}_i^t$, $\bar{P}_j^t$ the prestige of contributor $i$ and beneficiary $j$ when the transfer $x_{ij}^k$ is taking place upon time-slot $t > k$. Then:
\begin{align*}
\bar{P}_i^t+\bar{P}_j^t&=P_i^{k-1}-x_{ij}^k+ \sum\limits_{q=k}^{t}\delta \bar{P}_i^q+P_j^{k-1}+x_{ij}^k+ \sum\limits_{q=k}^{t}\delta \bar{P}_j^q,\\
%&=P_i^{k-1}+ \sum\limits_{q=k}^{t}\delta \bar{P}_i^q+P_j^{k-1}+ \sum\limits_{q=k}^{t}\delta \bar{P}_j^q,\\
&=P_i^{k-1}+C_i-d (P_i^{k}-x_{ij}^k)+\sum\limits_{q=k+1}^{t}\delta \bar{P}_i^q+P_j^{k-1}+ C_j-d (P_j^{k}+x_{ij}^k)+\sum\limits_{q=k+1}^{t}\delta \bar{P}_j^q,\\
&=P_i^{k}+\sum\limits_{q=k+1}^{t}\delta \bar{P}_i^q+P_j^{k}+\sum\limits_{q=k+1}^{t}\delta \bar{P}_j^q,\\
\vdots\\
&=P_i^t+P_j^t.\\
\end{align*}That is, prestige transfers do not affect the total prestige that exists in the system.
\end{proof}
The result of proposition 2 can be easily extended for the general case of $N$ users and all time-slots.

\begin{theorem}In progressive mining, users cannot retain more prestige by splitting their coins into multiple identities.
\end{theorem}
\begin{proof}Without loss of generality assume that user $i$ divides her coins into 2 identities according to $C_{i,1}$ and $C_{i,2}$, such that $C_{i,1}+C_{i,2}=C_{i}$. hen, the prestige retained by the multiple identities of user $i$ out of the prestige transferred from user $j$, $x$, will be:
\begin{align*}
f_{retain,1}(x)-x+f_{retain,2}(2x-f_{retain,1}(x))&=x\frac{P_{i,1}}{P_{i,1}+bP_{i,2}+P_b^i}-x+
\\&x\left(2-\frac{P_{i,1}}{P_{i,1}+b P_{i,2}+P_b^i}\right)\frac{P_{i,2}}{P_{i,2}+P_b^i},\\%\leq\\
%x_{ji}\left(\frac{P_{i,1}}{P_{i,1}+P_{i,2}+P_b^i} +\frac{P_{i,2}+P_b^i}{P_{i,1}+P_{i,2}+P_b^i}\frac{P_{i,2}}{P_{i,2}+P_b^i}\right)&=
%x_{ji}\frac{P_{i,1}+P_{i,2}}{P_{i,1}+P_{i,2}+P_b^i}\\
%&=x_{ji}\frac{P_{i}}{P_{i}+P_b^i}\\
&=x\frac{P_{i,1}P_{i,2}+P_{i,2}P_{b}^i+bP_{i,2}^2-bP_{i,2}P_{b}^i-(P_{b}^{i})^2}{(P_{i,1}+b P_{i,2}+P_b^i)(P_{i,2}+P_b^i)},\\
&\leq x\frac{P_{i,1}+P_{i,2}}{P_{i,1}+P_{i,2}+P_b^i},\\
&=x\frac{P_{i}}{P_{i}+P_b^i}\\
&=f_{retain(x)}.
\end{align*}where the inequality applies since:
\begin{align*}
\frac{P_{i,1}P_{i,2}+P_{i,2}P_{b}^i+bP_{i,2}^2-bP_{i,2}P_{b}^i-(P_{b}^{i})^2}{(P_{i,1}+b P_{i,2}+P_b^i)(P_{i,2}+P_b^i)}&\leq\frac{P_{i,1}+P_{i,2}}{P_{i,1}+P_{i,2}+P_b^i}\Longleftrightarrow
\\-P_{b}^i\left( bP_{i,1}P_{i,2}+P_{i,1}P_{b}^i+P_{i,2}(bP_{i,2}+P_{b}^i+bP_{b}^i)+(P_{b}^i)^2\right)&\leq P_{i,1}(P_{i,1}P_b^i+bP_{i,2}P_b^i+(P_b^i)^2).
\\
\end{align*}On the other hand, as we show in the proof of Theorem 1, $P_{i,1}+P_{i,2}=P_i$ and therefore the third equality is valid. Therefore, there is no prestige gain when a user creates multiple identities in progressive mining, intuitively due to the prestige payments that is forced to submit to her fake identities that in turn they retain only a portion of the prestige.

\end{proof}

\section{Composite Signatures}\label{sec:composite-sig}
Composite signatures~\cite{saxena2014increasing} are aggregate signatures satisfying the properties of \first \emph{incremental composition}, \second \emph{one-way}, and \third \emph{no-ordering}. \emph{Incremental composition} means that a number of individual signatures can be combined into a single signature, and more signatures can be added to the composite at any time; \emph{one-way} refers to the computational difficulty to obtain any sub-composite of signatures from only the composite signature; and \emph{no-ordering} means that the composite signature does not maintain the order of the individual signatures composing it.

We adopt the definition of composite signature schemes given by Saxena~\etal~\cite{saxena2014increasing}. Let's consider a message-descriptor $l$ made of pairs of (message,verification key): $l = \{(m_1 ,vk_1 ), \dots , (m_i ,vk_i )\}$. A composite signature scheme $\textbf{SIG}$ is defined by the set of algorithms below:
\begin{itemize}
\item \functiondef{SIG.Setup($1^\lambda$)}{$params$} defines the system parameters $params$ with respect to the security parameter $\lambda$. These parameters are publicly available.

\item \functiondef{SIG.Gen($params$)}{$sk,vk$} generates their secret key $sk$ and verification key $vk$ from the public $params$.

\item \functiondef{SIG.Sign($sk,m$)}{$\sigma$} outputs a single signature $\sigma$ on the message $m$ computed from the secret key $sk$.

\item \functiondef{SIG.Verify($l,\sigma$)}{$b$} takes as input a message-descriptor $l$ and a signature $\sigma$. Outputs a decision bit $b$ about the validity of the signature if all the messages in $l$ are unique; otherwise, it produces output: $invalid$.

\item \functiondef{SIG.Compose($(l_1,\sigma_1),(l_2,\sigma_2)$)}{$\sigma$} takes as input two pairs of (message-descriptors, signatures): $(l_1 ,\sigma_1 )$ and $(l_2 ,\sigma_2)$. Outputs the composite signature $\sigma$ on the message descriptors $l_1 \cap l_2$ if
\algo{Sig.Verify($l_1,\sigma_1$)} = $valid$ and \algo{Sig.Verify($l_2,\sigma_2$)} = $valid$, and $l_1 \cap l_2 = \emptyset$; otherwise outputs $\perp$.
\end{itemize}

%An interesting property of composite signatures is that an adversary cannot extract any individual signature from a composite signature~\cite{saxena2014increasing}.

Saxena~\etal~\cite{saxena2014increasing} propose a provably secure composite signature scheme but whose signature size increases linearly with the number of compositions. They also posit that BGLS signatures~\cite{bgls} satisfy the definition of composite signatures under a weaker security assumption~\cite{saxena2014increasing}. In this paper, we use BGLS as composite signature scheme as its signature size remains constant with the number of compositions.
